# Supplementary material for: Signal Convolution Logic
Source: arXiv:1806.00238 source file (2018-09-17)
Supplement: Supplementary file 1 [file appendix1.tex]

% !TEX root =  main.tex
\setcounter{theorem}{0}
\section{Soundness and Correctness: proofs}
\label{app:proofs}
In this appendix we report the proofs of the soundness and correctness of the quantitative semantics of SCL with respect to the Boolean semantics. To be clear, we report again also the statements of the theorems.

\begin{theorem}[Soundness Property]
\label{th:soundness}
	The quantitative semantics is sound with respect to the Boolean semantics, than means:
	$$
		\rho(\vec{s},t, \phi) > 0 \implies (\vec{s},t) \models \phi 
       \qquad and \qquad 
		\rho(\vec{s},t, \phi) < 0 \implies (\vec{s},t) \not \models \phi
$$
\end{theorem}
%	\begin{proof}
%    The demonstration is by induction on the structure of the formula. The soundness holds for the atomic predicates and boolean operators: this is the proof of soundness robustness, see \cite{robust1,fainekos-robust}. Consider then the  formula $\langle k_T, p\rangle \phi$. If $\rho(\vec{s},t, \langle k_T, p\rangle \phi) > 0$, by Definition \ref{def:quantiative_semantics} (Equation \ref{def:qs:4}) we have that $k_T * [\rho(\vec{s},\tau,\phi) > 0] > p$. 
%    %$k_T * \chi(\rho(\vec{s},t,\phi) > p$. 
%    By the inductive hypothesis, $\phi$ satisfies the soundness property, hence it follows that 
%    $[\rho(\vec{s},\tau,\phi) > 0] \equiv \chi(\vec{s},\tau, \phi)$
%   %  $(\vec{s},t) \models \phi$. 
%     It means that  $k_T * \chi(\vec{s},\tau, \phi) > p$ i.e., $(\vec{s},t) \models \langle k_T, p\rangle \phi$. \qed
%	\end{proof}
\begin{proof}
	The demonstration is by induction on the structure of the formula. The soundness holds for the atomic predicates and Boolean operators: this is the proof of soundness of {\it Metric Interval Temporal Logic} (MITL), see \cite{robust1,fainekos-robust}. 
Let us consider the formula $\langle k_T, p\rangle \phi$, with $\phi$ satisfying correctness by induction.
If $\rho(\vec{s},t, \langle k_T, p\rangle \phi) > 0$, by Definition \ref{def:quantiative_semantics} (Equation \ref{def:qs:4}) we have that $k_T(t) * [\rho(\vec{s},t,\phi) > 0 ] \ge p$. By the inductive hypothesis, $\phi$ satisfies the soundness property, hence it follows that $k_T(t) * \chi(\vec{s},t, \phi) \ge p$, i.e. $(\vec{s},t) \models \langle k_T, p\rangle \phi$. \qed
\end{proof}

%\todo{R1, Section 4.2, Definition 5, I cannot find what is the meaning of $sup$}

\begin{theorem}[Correctness Property] 
\label{th:correctness}
	The quantitative semantics $\rho$ satisfies the correctness property with respect to the Boolean semantics if and only if, for each formula $\phi$, it holds:
	\[  \forall \vec s_1,\vec s_2 \in \mathcal{D}(\mathcal{T};\mathcal{S}),\, \|\vec s_1-\vec s_2\|_\phi<\rho(\vec{s}_1,t,\phi)  \Rightarrow \chi(\vec s_1,t, \phi)=\chi( \vec s_2,t, \phi)
  \]	
% 	If the previous property is true for all the formulas of the language we say that the quantitative semantics satisfies the correctness property for the entire language.
\end{theorem}

    \begin{proof}
    We proceed by induction on the structure of the formula.  The correctness holds for  atomic predicates and Boolean operators by the correctness proof of quantitative semantics for {\it Metric Interval Temporal Logic} (MITL)~ \cite{fainekos-robust}.
    Let us consider the formula $\psi = \langle k_T, p\rangle \phi$, with $\phi$ satisfying correctness by induction. Let $\vec s_1$ and $\vec s_2$ be two signals  satisfying the hypothesis of the theorem, $\hat r = \rho(\vec{s}_1,t,\psi)$ and $\chi(\vec s_1,t, \psi)=1$ (the case $\chi(\vec s_1,t, \psi)=0$ is similar). We have to prove that $\chi(\vec s_2,t, \psi)=1$.
    
The hypothesis $\hat r = \rho(\vec{s}_1,t,\psi)$ implies that $k_T *  [\rho(\vec{s}_1,t,\phi)  > \hat r]  \ge p$. This means that $\exists P\subseteq t+T$ s.t. 
  $$\forall \tau \in P,\, \rho(\vec{s}_1,\tau,\phi) > \hat r =\rho(\vec{s}_1,t,\psi) >  \|\vec s_1-\vec s_2\|_\phi =\|\vec s_1-\vec s_2\|_\psi$$ ( the last equal holds because $\psi$ and $\phi$ have the same atomic propositions). Then, for the inductive hypothesis,  $ \forall \tau \in P,\, \chi(\vec s_1,\tau, \phi)=\chi( \vec s_2,\tau, \phi)=1$ which clearly implies that $k_T *\chi(\vec{s}_2,\tau,\phi)\ge p$, i.e., $ \chi(\vec s_2,t, \psi)=1$.
%    $P$ corresponds to the (minimum) positive subset of $T$ for which $k_T *  [\rho(\vec{s}_1,t,\phi)  > \hat r]  >p$ but $\chi(\vec s_2,t,\phi) $ is positive in the same subset, this means that also  $k_T * \chi(\vec s_2,t,\phi) > p$.
    
%     We have to prove that $k_T * \chi(\vec s_2,t,\phi) > p$.
%    %$\mu_i (r,t) = [\rho((\vec{s}_i,t, \psi)  >r]$ for $i=1,2.$  
%    %$k_T * \mu_1(r,t) > p$ $\forall 0 \leq r \leq \hat r, $ and in particular $k_T * \chi(\vec s_1,t,\phi) = q \geq p$
%    We know that $k_T *  [\rho(\vec{s}_1,t,\phi)  > \hat r]  >p$. This means that 
%    $\exists P\subseteq T$ s.t. 
%    $$\forall t' \in P, \rho(\vec{s}_1,t'\psi) \geq \hat r =\rho(\vec{s}_1,t,\langle k_T, p\rangle \phi) >  \|\vec s_1-\vec s_2\|_\phi =\|\vec s_1-\vec s_2\|_\psi$$ ($\phi$ and $\psi$ have the same atomic propositions). Then, for the inductive hypothesis,  $ \chi(\vec s_1,t', \phi)=\chi( \vec s_2,t', \phi)=1, \forall t' \in P.$ 
%    P corresponds to the (minimum) positive subset of T for which $k_T *  [\rho(\vec{s}_1,t,\phi)  > \hat r]  >p$ but $\chi(\vec s_2,t,\phi) $ is positive in the same subset, this means that also  $k_T * \chi(\vec s_2,t,\phi) > p$.

    % there exists a set $P\subseteq T$ such that $(k_P*1(\rho(\phi,s,t)))(t)$ $\frac{|P|}{|T|}>p \mbox{ and } \forall t'\in P,\, \rho(\vec{s}_1,t',\langle k_T, p\rangle \psi) = r$. For inductive hypothesis $\phi$ satisfies the correctness property meaning that  $\forall t'\in P,\, (\vec s_2, t') \models \langle k_T, p\rangle \psi$ but this implies that $(\vec s_2, t) \models \langle k_T, p\rangle \langle k_T, p\rangle \psi$.  
\end{proof}

\newpage
