# Supplementary material for: Signal Convolution Logic
Source: arXiv:1806.00238 source file (2018-09-17)
Supplement: Supplementary file 2 [file appendix2.tex]

% !TEX root =  main.tex
\section{Monitoring Algorithm: details}
\label{app:monitoring}
In this section we detail the first monitoring algorithm presented in Section \ref{sec:monitoring}, 
showing how to efficiently implement the computation sketched in the above mentioned section. 

Let us denote with $\mathcal{M}_{\phi}$ the monitoring algorithm (monitors) of $\phi$. It produces as output tuple $\{(t_i,b_i) \}_{i\ge 0}$ which are stored directly into two buffer queues $qT_\phi$ and $qB_\phi$. The first queue contains the times $\{t_i\}_{i\ge 0}$ and the second queue contains the boolean values $\{b_i\}_{i\ge 0}$ such that if $b_i = 1$ than $ \forall t \in [t_i,t_{i+1}),\,(t, \vec s) \models \phi$, otherwise if $b_i = 0$  than $ \forall t \in [t_i,t_{i+1}),\,(t, \vec s) \not \models \phi$. This queues are than shared to other monitors which need the values stored in, for example the algorithm $\mathcal{M}_{\phi_1 \wedge \phi_2 }$ can access to $qT_{\phi_1}$,$qB_{\phi_1}$,$qT_{\phi_2}$,$qB_{\phi_2}$.  
In Algorithm~\ref{alg:monitoring} we show the monitor of formulas with temporal operator $\langle k_{[T_0,T_1]}, p \rangle \phi$. The monitors of other kind of formulas are standard.

Let us consider the monitor $ \mathcal{M}_{\langle k_{[T_0,T_1]}, p \rangle \phi}$ (Algorithm \ref{alg:monitoring}). It is composed by three phases. The \emph{initialization phase} (line $2-9$) where the algorithm  waits until the first change of truth value of the signal occurs inside the convolution windows (i.e $[t+T_0,t+T_1]$). The \emph{storing phase} (line $10 - 16$) where the algorithm stores information until a truth change outside the convolution windows occurs. The \emph{evaluation phase} (line $17 - 33$) where the algorithm is ready to calculate the boolean semantics in $t$ and for the next truth change until the final monitoring time ($t_{end}$) is met.

In the initialization phase, after setting the variables, a while loop (line $5 - 8$) is performed. Its purpose is to initialize the $b_i$ variable to the values of the boolean semantics of $\phi$ evaluated in $t_i = t+K.T_0$. 

In the storing phase, which starts in line $10$, the monitor moves the elements from the queue $qT_{\phi}$,$qB_{\phi}$ to the internal queues \texttt{time} and \texttt{space}, respectively, until the time obtained by $qT_{\phi}$ is outside of the convolution windows (see the while condition at line 10). During the storing phase the threshold variables \texttt{th} is updated (line $14$) and the variables $\mathtt{b_f}$ points to boolean semantics of $\phi$ evaluated in $\mathtt{t_f}= \mathtt{t}+\mathtt{K.T_1}$.  The variable \texttt{th} is related to the monitoring of $ \langle k_{[T_0,T_1]}, p \rangle \phi $. A positive values means that  $ \langle k_{[T_0,T_1]}, p \rangle \phi $ is satisfied. On the contrary, a negative values means  $ \langle k_{[T_0,T_1]}, p \rangle \phi $ is not satisfied. For this reason,  the simple idea of this online monitoring algorithm consists in monitoring when $\mathtt{th}$ changes sign.At the end of the storing phase we are able to produce the output of the monitor in time \texttt{t} and moving the convolution windows to the right so to evaluate the boolean semantics for $t> \texttt{t}$. 

When we enter into the evaluating phase (line $20$), we have two internal queues  \texttt{time} and \texttt{space} which store all the necessary data to update the threshold $\mathtt{th}$ and consequently to calculate the boolean semantics of the target formula. There are two pointers $\mathtt{t_i}$ which points to a time before the first elements stored in  $\texttt{time}$ and $\mathtt{t_f}$ which points to the last element stored in $\texttt{time}$. The interval $[\mathtt{t_i},\mathtt{t_f}]$ represents the time window in which it is necessary to apply the convolution in order to compute the boolean semantics of the formula $\phi$ in $\mathtt{t}$. As soon as a new tuple arrives $(t_{new},b_{new})$ we are able to move the convolution windows from  $[\mathtt{t_i},\mathtt{t_f}]$ to $[\mathtt{t_i}+h,\mathtt{t_f}+h]$ where $h=t_{new} - \mathtt{t_f}$. It means that the algorithm is able to monitor the boolean semantics from $\mathtt{t}$  to $\mathtt{t_i}+h$. The idea is to check during this translation to the right if and the exact moment when the variables \texttt{th} changes sign. 
This entire procedure is achieved by the while loop (line $21 - 36$). 
This is achieved by the method \textsc{solve} in line 24 and 30. As we noticed the translation is not performed in a row but there are two cases [\ldots]. The monitoring algorithm is than performed until the the specified time ($t_{end}$) is reached (see the while-loop condition at line 20)

\begin{algorithm}[ht]
\caption{}\label{alg:monitoring}
\begin{algorithmic}[1]
\Procedure{monitor($t,kernel,p$)}{}
\State $\mathtt{t} \gets t,\,\mathtt{K} \gets kernel,\,\mathtt{t_f} \gets t,\,\mathtt{th} \gets -p$
\State $\mathtt{signal} \gets [],\,\mathtt{time} \gets [],\,\mathtt{qT} \gets qT,\,\mathtt{qB} \gets qB$
\State $ t_{new} \gets \mathtt{t}  $
\While{ ($t_{new}\le \mathtt{t}+\mathtt{K.T_0}$)}
\State $b_{i} \gets \text{\texttt{qB}.pop()}$
\State $ t_{new} \gets \text{\texttt{qT}.pop()}  $
\EndWhile
\State $\mathtt{t_i} \gets \mathtt{t}+\mathtt{K.T_0}$
\State $\mathtt{t_{app}} \gets \mathtt{t_i}$
%\State $b_{new} \gets b_{new}$
%\State \texttt{time}.push($\mathtt{t}+\mathtt{K.T_0}$)
%\State \texttt{signal}.push($b_{new}$)
%\State $b_{new} \gets \texttt{qB}.pop()$
\While{ ($t_{new}\le \mathtt{t}+\mathtt{K.T_1}$)}
\State \texttt{time}.push($t_{new}$)
\State \texttt{signal}.push($b_{new}$)
\State $\texttt{th} \gets \texttt{th} + \mathtt{b_f} \cdot \text{\texttt{K}.integrate}(\mathtt{t_{app}} - \mathtt{t_i},t_{new}-\mathtt{t_i} )$
\State $\mathtt{t_{app}} \gets t_{new}$
\State $\mathtt{b_f}\gets b_{new}$
\State $ (t_{new},b_{new}) \gets (\text{\texttt{qT}.pop()}, \text{\texttt{qB}.pop()}$)
\EndWhile
\State $\mathtt{t_f}\gets \mathtt{t}+\mathtt{K.T_1} $
\While{$\mathtt{t_f} < t_{end}$ }
\While{ $\mathtt{t_f} < t_{new}$}
\If{ ($\text{\texttt{time}.peek()}-\mathtt{t_i}\le t_{new} - \mathtt{tf}$)}
\State $h \gets (\text{\texttt{time}.peek()}-\mathtt{t_i})$
\State $\texttt{th} \gets \textsc{solve}(\texttt{th},h,\mathtt{b_i},\mathtt{b_f},\mathtt{K})$
\State $\mathtt{t_i} \gets \text{\texttt{time}.pop()}$
\State $\mathtt{b_i} \gets \text{\texttt{signal}.pop()}$
\State $\mathtt{t_f} \gets  \mathtt{t_f} + h $
\Else
\State $h \gets t_{new} - \mathtt{tf}$
\State $\texttt{th} \gets \textsc{solve}(\texttt{th},h,\mathtt{b_i},\mathtt{b_f},\mathtt{K})$
\State $\mathtt{t_i} \gets \mathtt{t_i}+ h $
\State $\mathtt{t_f} \gets  t_{new} $
\State $\mathtt{b_f} \gets  b_{new} $
\EndIf
\State $\texttt{t} \gets \texttt{t} + h$
\EndWhile
\State $ (t_{new},b_{new}) \gets (\text{\texttt{qT}.pop()}, \text{\texttt{qB}.pop()}$)
\EndWhile
\EndProcedure

\end{algorithmic}
\end{algorithm}
