# Supplementary material for: Signal Convolution Logic
Source: arXiv:1806.00238 source file (2018-09-17)
Supplement: Supplementary file 3 [file appendix3.tex]

\section{Monitoring Algorithm: details}
\label{app:monitoring}

\begin{algorithm}[ht]
\caption{Efficient Convolution Algorithm 
% $(K_T * U)(t)$ 
$\chi ( \vec s , t,\langle k_{[T_0,T_1]}, \delta,  p \rangle \phi)$
}\label{alg:monitoring}
\begin{algorithmic}[1]
\Require{$t_{i},t_{e},k_{[T_0,T_1]},\chi ( \vec s , t, \phi),p$}
% \State $\textsc{initialize}(H(t_{i}))$
% \State $\textsc{initialize}(init,end)$
\State $U \gets \textsc{Decompose}(\chi ( \vec s , t, \phi) $
\State $H(t_{i})= (K_{[T_0,T_1]} * U)(t_{init})$
\State $\textsc{initialize}(init,end)$
%$(K_T * y)(t_{init})$
%\State $[U^0_0,U^0_1]$ s.t. $\chi ( \vec s , t, \phi) = 1, \forall t \in [U^0_0,U^0_1]$ and $0$ otherwise
\item[]
\While{($t<t_{e}$)}
\If{ ($t+T_0 \in U^{init} \textbf{ and } t+T_1 \in U^{end}$)}
\State $\delta_{step} \gets \min(\delta,t+T_0-U^{init}_1,U^{end}_1-t-T_1)$
\State $\Delta H \gets K_T(T_0) - K_T(T_1) + \sum_{i=init+1}^{end-1} ( k_T(U^{i}_0-t) - k_T(U^{i}_1-t))$
\EndIf
\If{ ($t+T_0 \in U^{init} \textbf{ and } t+T_1 \not\in U^{end}$)}
\State $\delta_{step} \gets \min(\delta,t+T_0-U^{init}_1,U^{end+1}_0-t-T_1)$
\State $\Delta H \gets K_T(T_0)  + \sum_{i=init+1}^{end} ( k_T(U^{i}_0-t) - k_T(U^{i}_1-t))$
\EndIf
\If{ ($t+T_0 \not\in U^{init} \textbf{ and } t+T_1 \in U^{end}$)}
\State $\delta_{step} \gets \min(\delta,U^{end}_1-t-T_1,U^{init}_0-t-T_0)$
\State $\Delta H \gets  -K_T(T_1)  + \sum_{i=init}^{end-1} ( k_T(U^{i}_0-t) - k_T(U^{i}_1-t)) $
\EndIf
\If{ ($t+T_0 \not\in U^{init} \textbf{ and } t+T_1 \not\in U^{end}$)}
\State $\delta_{step} \gets \min(\delta,U^{init}_0-t-T_0,U^{end+1}_0-t-T_1)$
\State $\Delta H \gets \sum_{i=init}^{end} ( k_T(U^{i}_0-t) - k_T(U^{i}_1-t)) $
\EndIf
\item[]
\State $H(t +\delta_{step}) \gets H(t)+\delta_{step}\cdot\Delta H$
\If{$(H(t +\delta_{step})-p)\cdot(H(t)-p)\le0)$}
\State $\textsc{find}(\{x \in [t,t+\delta_{step}] \mid H(t +x)-p=0\})$
\EndIf
\State $t \gets t+\delta_{step}$
\If {($t+T_0\ge U^{init}_1$)}
\State $init \gets init+1$
\EndIf
\If{($t+T_1\le U^{end}_1$)}
\State $end \gets end+1$
\EndIf
\EndWhile
%\EndProcedure
\end{algorithmic}
\end{algorithm}
We now describe Algorithm~\ref{alg:monitoring}, which  efficiently evaluates the convolution between a generic kernel, $k_T$,  and a Boolean signal $\chi ( \vec s , t, \phi)$.  The Boolean signal can be decomposed \cite{MalerN04} in a sequence of disjoint unitary signals $U = U^1 + \dots + U^n$ s.t. each $U^i(t)$ is true only in a single interval of time  $[U^i_0,U^i_1]$, false outside.
%Let us calling 
%$U=\{[U^0_0,U^0_1], \dots, [U^n_0,U^n_1] \} $ the interval covering of the signal, corresponding to the set of disjoint interval where the signal is true, then, $\forall i \le n$ 
%$U^i(t) = 1,$ iff $t \in  [U^i_0,U^{i}_1)$ and zero otherwise.
%We denote with U^i_0,U^i_1 

The algorithm takes as inputs the interval $[t_{i},t_{e}]$ where to evaluate the boolean semantics of $\chi ( \vec s , t,\langle k_{[T_0,T_1]}, p \rangle \phi)$ , the kernel $k_{[T_0,T_1]}$, the Boolean signal $\chi ( \vec s , t, \phi)$, 
the maximum allowed integration step $\delta$, and the threshold $p \in [0,1]$.

The algorithm (line 1) decomposes the Boolean signal $\chi ( \vec s , t, \phi)$ into unitary signals as explain above, afterward  (line 2) it initializes $H(t_{i})$ to $(K_{[T_0,T_1]} * U)(t_{i})$ which is evaluated by a standard integration technique, and the value of $init$ and $end$, which are two integers pointing to the first unitary signal of $U$ such that  $U^{init}_1  > t_i + T_0$, and  the last unitary signal such such that $U^{end}_0 \le t_i+T_1$.
The algorithm then performs the integration of the ODE defined in Equation \eqref{eq:generalODEpositiveInterval} by considering only the unitary signal composing $U$ which intersect ($t+[T_0,T_1]$). A while cycle (line $4 - 32$) performs the integration step until the convolution is evaluated on the entire interval $[t_{i},t_{e}]$. Depending on the cases, if the bounds of the convolution window(i.e., $t+T_0$ and $t+T_1$) intersect an unitary signal composing $U$, four different integration strategies are performed (blocks at lines: $5-8,9-12,13-16,17-20$), and the proper value of the integration steps (i.e $\delta_{step}$) which avoids discontinuity is also evaluated (lines: $6,10,14,18$). The value of $\delta_{step}$, indeed, implies that between  $t$ and $t+\delta_{step}$ no new intersection of unitary signals $U^i$ with the convolution windows occur.   Afterward, the approximation of the finite difference $H(t+\delta_{steps}) - H(t)$ is stored in $\Delta H$ and the integration step ($H(t+\delta_{step}) =  H(t) + \delta_{step} \cdot \Delta H$) is performed (line 21). If during this integration step $H(t)-p$ changes sign (line 22), then the exact moment is evaluated by means of a root finding routine (line 23). These time values define the Boolean semantics of $\chi ( \vec s , t,\langle k_{[T_0,T_1]}, \delta,  p \rangle \phi)$.   Finally, in lines $25-30$, the values of t,  $init$ and $end$ are updated and the cycle continues.

The time-complexity of the algorithm for the convolution operator is proportional to the computational cost of numerically integrating the differential equation above. Using a solver with constant step size $\delta$, the complexity is proportional to the number of integration steps, times the number $N_U$ of unitary components in the signal: $O((T_s/\delta)N_U)$. By fixing the precision of the integrator to $\delta$, the number $N_U$ of unitary components is itself bounded by $(T_s/\delta)$. This is because the integral, being sampled at $\delta$ units of time, cannot cross the threshold $p$ more than once in each $\delta$-time interval. It follows that   $O(T_s/\delta)$ is an upper bound on $N_U$ for any signal $\chi(\vec{s},t,\phi)$ encountered in the monitoring procedure. This gives a complexity upper bound of the order or $O((T_s/\delta)^2)$ for each convolution operator of a formula. Considering that the time-complexity of the other logical operators is bounded by $O(N_U) = O((T_s/\delta))$ (see \cite{robust2}), we conclude that for a  formula of size $M$ (i.e. having $M$ logical operators) and  integration step  $\delta$, the complexity of monitoring  is $O(M(T_s/\delta)^2)$.
